# Supplementary material for: Specialised or Generic? Tokenization Choices for Radiology Language Models
Source: arXiv:2508.09952 ancillary file (2025-08-13)
Supplement: Supplementary file 1 [file suplementary_materials.pdf]

# Supplementary Materials

## 1 Methods: Memory calculation extended

**Vocabulary, sequence length and computation constraints:** This section goes into more detail to explain how we derive an estimate of the GPU memory required during LM training in the main paper. A calculation of the GPU memory required for a transformer-based LM depends on the model's vocabulary size $V$, input sequence length $S$, the batch size $B$, the models dimensions $D$, number of heads $H$, and number of transformer blocks $N$.

An approximation of the memory required by a transformer decoder in a single training step is:

$$M = M_{\text{act}} + M_{\theta} + M^{\theta}_{\text{grad}} + M_{\text{opt}} \tag{1}$$

where $M_{\text{act}}$ is the memory required to store intermediate activations during the forward pass, $M_{\theta}$ is the memory of storing the model parameters $\theta$, $M^{\theta}_{\text{grad}}$ is the memory required to store the gradients of $\theta$, and $M_{\text{opt}}$ is the memory required to store the optimizer states [2]. This does not take into account "temporary" memory used for matrix operations of attention or linear layers as these are dependent on library-specific implementations and unloaded from memory after their calculation. In contrast, storage of activations, parameters, gradients and optimization state has to be persistent throughout the whole training step, thus considered. Memory for activations $M_{\text{act}}$ is calculated as:

$$\begin{aligned} M_{\text{act}} = &\underbrace{BSV}_{\text{Lin. proj.}} + N\Big[\underbrace{BSD}_{\text{LN}} + \underbrace{5(BSD) + 2(BS^2H)}_{\text{MHA}} + \underbrace{BSD}_{\text{LN}} + \underbrace{(BSD + 8(BSD))}_{\text{FFN}}\Big] \\ &+ \underbrace{BSD}_{\text{LN}} + \underbrace{BSD}_{\text{Lin. proj.}} + \underbrace{BSV}_{\text{Loss}}, \end{aligned} \tag{2}$$

which simplifies to Eq. 2 in the main paper:

$$M_{\text{act}} = 2BSV + 2BSD + N\Big[16BSD + 2(BS^2H)\Big]. \tag{3}$$

Here, $LN$ refers to layer normalisation, $FFN$ is the feedforward layer in the transformer block, $MHA$ is the multi-head attention block, and Lin.proj. the linear projections.

$M_{\theta}$ is given by:

$$M_{\theta} = \underbrace{DV}_{Lin.Proj.} + N\Big[\underbrace{2D}_{LN} + \underbrace{4D^2}_{\text{MHA}} + \underbrace{8D^2}_{\text{FFN}}\Big] + \underbrace{D}_{LN}, \tag{4}$$

The memory $M^{\theta}_{grad}$ required for storage of gradients of the loss with respect to all parameters is $M^{\theta}_{grad} = M_{\theta}$, because one gradient per parameter must be retained in memory until the optimiser update is applied to all parameters simultaneously at the end of a training step. We do not consider gradients with respect to the activations as these are computed layer by layer during back-propagation and continuously discarded making their memory contribution transient.

$M_{opt}$ depends on the optimiser used. Adam takes more memory than SGD, as it needs to store both the time averaged momentum and the variance of the gradients. For Adam, used in our study,

$$M_{opt\ Adam} = 2 \times M_{\theta}.$$

The memory for storing the model parameters $M_{\theta}$, gradients $M_{\text{grad}}$ and optimizer state $M_{\text{opt}}$ is small compared with the memory for activations $M_{\text{act}}$ for non-trivial values of batch size $B$ ($\sim 1\%$) [2] (as can be seen in Fig. 2b of the main paper).

A key contributor to memory usage is the attention mechanism, typically implemented as scaled dot-product attention,

$$\text{Attention}(Q, K, \mathcal{V}) = \text{softmax}\left(\frac{QK^T}{\sqrt{d_k}}\right)\mathcal{V}, \tag{5}$$

where $Q$, $K$, and $\mathcal{V}$ are the query, key, and value matrices respectively, and $d_k = D/H$ is the dimensionality per attention head in a multi-head attention (MHA) layer. This gives the quadratic dependence of $M$ on $S$ in Suppl. Eq. 3.

## 2 Additional experimental details

In this section additional details required to train the models presented in our paper are provided. The model configurations - batch sizes $B$, vocabulary $V$ and maximum sequence lengths $S$ - used to train the LM for each experiment are given in Tab. 1. In these configurations, defined for experiments that evaluate performance of LMs with different tokenizers, we adjusted batch-size B for each setting such that most of GPU memory is utilized during training by the batch (e.g. LMs using *General* tokenizers require more memory for 1 sample, so they can fit smaller batches in the same memory than LMs using other Tokenizers). The models were trained for 50 epochs, using cross entropy loss and the AdamW optimiser. Where given, the official train, validation and test splits of the public datasets are used to train the LM.

The theoretical memory (main paper Fig 2b) is calculated from Eq. 1 for the specific model configurations (Tab. 1 herein) but with constant $B = 32$ for a straightforward comparison of memory required by different tokenizers for the same number of samples. The value $B = 32$ is the maximum value possible to fit for an LM using the *General* tokenizer for CT-RATE and PET-CT, so it is

**Table 1:** Model configurations for BPE vocabularies. The General tokenizer for all datasets is the GPT2 tokenizer. The medical tokenizer is trained on PubMed abstracts. Domain specific tokenizers are trained only on the train split of the evaluation dataset.

| Eval. Dataset | Domain | Vocab. size | Sequence Length | Batch size |
|---|---|---|---|---|
| MIMIC | Specific | 9.1k | 256 | 128 |
| | Medical | 30k | 512 | 128 |
| | General | 50k | 512 | 64 |
| CT-RATE | Specific | 9.4k | 512 | 128 |
| | Medical | 30k | 512 | 128 |
| | General | 50k | 1024 | 32 |
| PET-CT | Specific | 11.0k | 512 | 128 |
| | Medical | 30k | 512 | 128 |
| | General | 50k | 1024 | 32 |

deemed a representative number for comparison of memory savings with other tokenizers. As memory of activations (Eq. 3) is the main factor determining memory use (Fig.2 main paper) and it is linear with respect to $B$, the same trends are expected for other values of $B$. Theoretical memory for 1 sample ($B$=1) is shown in Fig 1. Finally, these memory calculations are based on storing numbers as data-type float32 - to convert $M$ calculated in Sec. 1 to the theoretical memory in main paper Fig. 2b is $4M/(1024^3)$. The use of mixed precision can lower the overall required memory but no change in trends are expected that would affect the arguments of the paper.

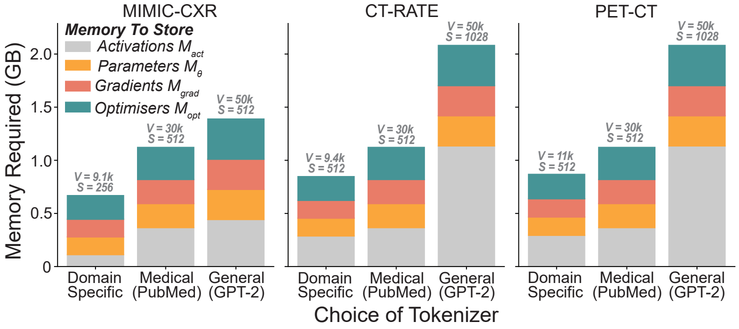


**Fig. 1:** Memory required to train LMs for the different tokenizers, calculated using Eq. 1 for 1 sample (B=1).

## 3 Experimental results: Additional information

For the F1 scores calculation from the extracted disease labels we follow prior work [1, 3, 5, 6], uncertain Chexbert labels are treated as positive and "not mentioned" as negative [4]. Macro-averaging gives equal weight to each class, while micro-averaging gives equal weight to each instance.

## References

1. Hou, B., et al.: Ratchet: Medical transformer for chest x-ray diagnosis and reporting. In: MICCAI (2021) 4
2. Korthikanti, V., et al.: Reducing activation recomputation in large transformer models (2022) 1, 2
3. Miura, Y., et al.: Improving factual completeness and consistency of image-to-text radiology report generation. NAACL-HLT (2021) 4
4. Smit, A., et al.: Combining automatic labelers and expert annotations for accurate radiology report labeling using BERT. EMNLP (2020) 4
5. Tanida, T., et al.: Interactive and explainable region-guided radiology report generation. CVPR (2023) 4
6. Warr, H., et al.: Quality Control for Radiology Report Generation Models via Auxiliary Auditing Components. MICCAI: UNSURE (2025) 4
